# Supplementary material for: Thermal spin wave noise as a probe for the Dzyaloshinkii-Moriya interaction
Source: arXiv:2502.03166 ancillary file (2025-02-05)
Supplement: Supplementary file 1 [file supplement.pdf]

# Supplemental Material: Thermal spin wave noise as a probe for Dzyaloshinkii-Moriya interaction

Aurore Finco,[1,*] Pawan Kumar,[1] Van Tuong Pham,[2] Joseba Urrestarazu-Larrañaga,[2] Rodrigo Guedas Garcia,[2] Maxime Rollo,[1] Olivier Boulle,[2] Joo-Von Kim,[3] and Vincent Jacques[1]

[1]*Laboratoire Charles Coulomb, Université de Montpellier, CNRS, Montpellier, France*
[2]*Université Grenoble Alpes, CNRS, CEA, SPINTEC, 38054 Grenoble, France.*
[3]*Centre de Nanosciences et de Nanotechnologies, CNRS, Université Paris-Saclay, 91120 Palaiseau, France*

## CONTENTS

I. Experiments on a single ferromagnetic layer 2

II. Evolution of the non-reciprocity with $D$ 4

III. Expected noise level at various probe heights 5

IV. Sample preparation 6

V. Calibration of the diamond probes 7

VI. Micromagnetics simulations 8
A. Geometry and parameters 8
B. Spin wave dispersion relations 9
C. Simulated magnetic noise spectra 9

References 9

* aurore.finco@umontpellier.fr

## I. EXPERIMENTS ON A SINGLE FERROMAGNETIC LAYER

As mentioned in the main text, the measurements are easier to perform and analyze on synthetic antiferromagnetic stacks, because of the strong reduction of the static stray field above the domain walls compared to a single ferromagnetic layer. Indeed, a domain wall in a very thin Co layer can easily produce a magnetic field of 10 to 15 mT, probed 60 nm away from the surface. Such a strong field induces a mixing of the spin states of the NV center and consequently a decrease of the PL signal [1] which adds up with the magnetic noise related PL decrease in the images. In addition, the ESR contrast is also significantly reduced, as well as the contrast in $T_1$ measurements. Nevertheless, we performed $T_1$ measurements on a single Co layer in a stack grown on a membrane, in order to confirm that the detected magnetic noise should indeed be significantly lower above a Néel right domain wall than above a Néel left domain wall.

Our stack is grown on a 25 to 30 nm-thick membrane, with the following composition: Ta (3 nm)|Pt (3 nm)|Co (1.35 nm)|Ru (0.85 nm)|Ta (2 nm). Looking at the sample from the top, we should observe Néel left domain walls, while when expect Néel right domain wall when measuring the bottom surface. During these experiments, we realized that diamond probes with parabolic pillars optimized for PL collection are not well adapted for scanning probe measurements on membranes, as they lead to strong oscillations in the AFM feedback signal and consequently in the PL, as visible in Fig. S1(d). Using flatter Quantilever MX probes from Qnami was more successful, despite their lower PL count rate.

These $T_1$ measurements are performed following the usual protocol: a first laser pulse is used to polarize the NV center in the bright state, before a variable time delay $\tau$ and then another laser pulse, which we use to read the state of the NV center. We obtain an exponential decay of the PL signal at the beginning of the readout pulse, with a decay constant which is directly $T_1$.

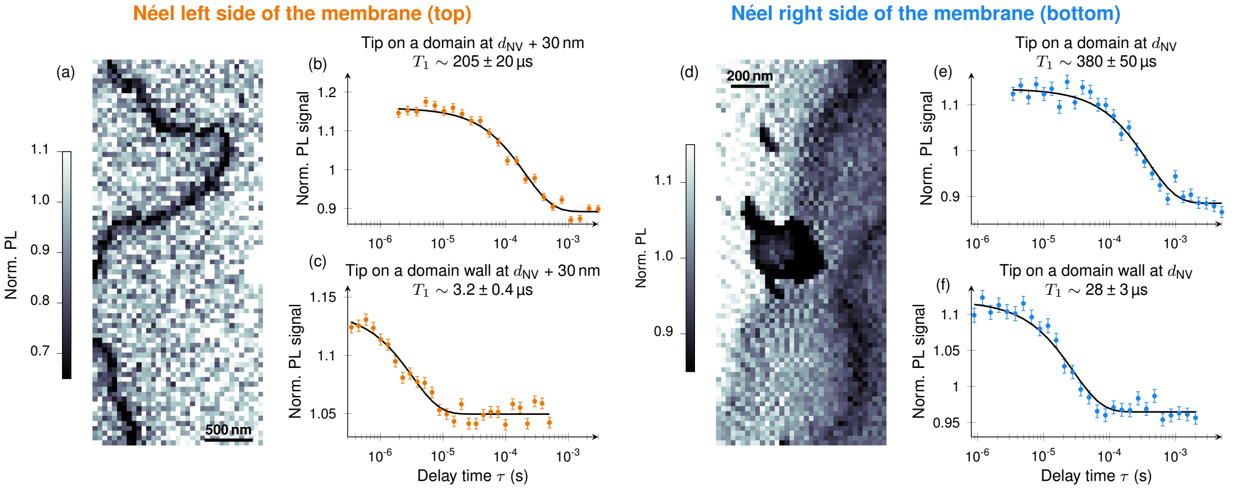


FIG. S1. (a) Image of a domain wall from the Néel left side. (b)-(c) $T_1$ measurements above a domain and above a domain wall, on the Néel left side of the sample, with the tip lifted 30 nm away from the surface. (d) Image of domain walls from the Néel right side. The large dark area in the center is a defect of the membrane. (e)-(e) $T_1$ measurements above a domain and above a domain wall, on the Néel right side of the sample.

We first localize a Néel left domain wall, looking at the sample from the top (Fig. S1(c)). It appears very clearly as a dark line in the PL map, as a result from the combined PL reductions originating from the static stray field and the magnetic noise. Figs. S1(b) and (c) display $T_1$ measurements above a domain and a domain wall. The tip was lifted 30 nm away from the surface, so that the measurement of the Néel right textures through the membrane will be performed at a similar distance from the magnetic layer. We observe a very strong decrease of $T_1$ above the wall ($T_1 = 3.2 \pm 0.4\,\mu s$) compared to above the domain ($T_1 = 205 \pm 20\,\mu s$), revealing the presence of a significant magnetic noise with a spectral component about 2.9 GHz, with a larger intensity in the domain walls. This situation is the same as in the SAF stack with Néel left domain walls.

Then we flip the sample and repeat the experiment on the bottom surface of the membrane, thus investigating Néel right textures. An image with two domain walls is presented in Fig. S1(d). Note that the PL gradient in the horizontal direction and the reduced image quality originate from the difficulty of scanning with the AFM on the membrane away from its edge. Nevertheless, we can clearly identify domain walls and repeat the $T_1$ measurements (Fig. S1(e)-(f)), with exactly the same tip as for the Néel left measurement. We still observe a decrease of $T_1$ above the domain ($T_1 = 380 \pm 50\,\mu s$) and again a further reduction above the domain wall ($T_1 = 28 \pm 3\,\mu s$). The effect is however significantly smaller than on the other side of the sample, in agreement with the theoretical prediction and the experiments on the SAF stack.

## II. EVOLUTION OF THE NON-RECIPROCITY WITH $D$

Figure S2 shows the computed dispersion relation of domain wall channeled spin wave modes for different values of the Dzyaloshinskii-Moriya constant. As discussed in Section VI, the dispersion relation is calculated from the transient response to a wavevector-dependent sinc RF field pulse, which is applied to a static, straight domain wall found from energy minimization. As $D$ is increased, we observe a stronger asymmetry in the dispersion, as expected from previous work [2].

For larger values of $D$, however, such as for $D = 1$ mJ/m$^2$ shown in the figure, we find that the straight domain wall is unstable with respect to long wavelength fluctuations, which is indicative of mode softening. This is reflected in Figs. 1(c) and S2 by an interval around $k = 0$ in which the dispersion curve is absent. Indeed, long time simulations for perturbations at these wavelengths show that the system evolves towards a labyrinthine domain structure, which is not seen for shorter wavelength excitations.

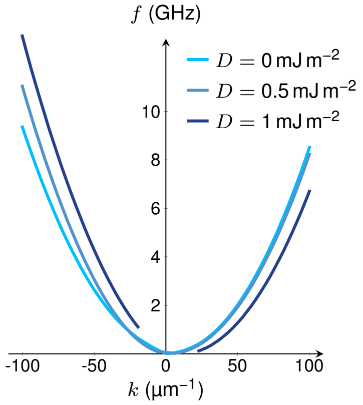


FIG. S2. Plot of the calculated spin wave dispersion inside a domain wall in the single Co layer of Fig. 1 of the main text, varying the DMI constant $D$. We observe an enhancement of the non-reciprocity with $D$, which we relate to the increase of the noise level difference between Néel left and right domain walls when increasing $D$.

## III. EXPECTED NOISE LEVEL AT VARIOUS PROBE HEIGHTS

Additional data accompanying Fig. 1(d) is presented in Fig. S3, where the maximum noise level detectable above a straight domain wall is shown as a function of $D$ for three probe heights.

The maximum noise level is calculated as follows. For a given noise map, such as those shown in Figs. 1(f) and 1(g), we compute an average over 16 horizontal line cuts of the noise profile. The maximum value of this average, which occurs approximately at the wall center, is reported in the figure.

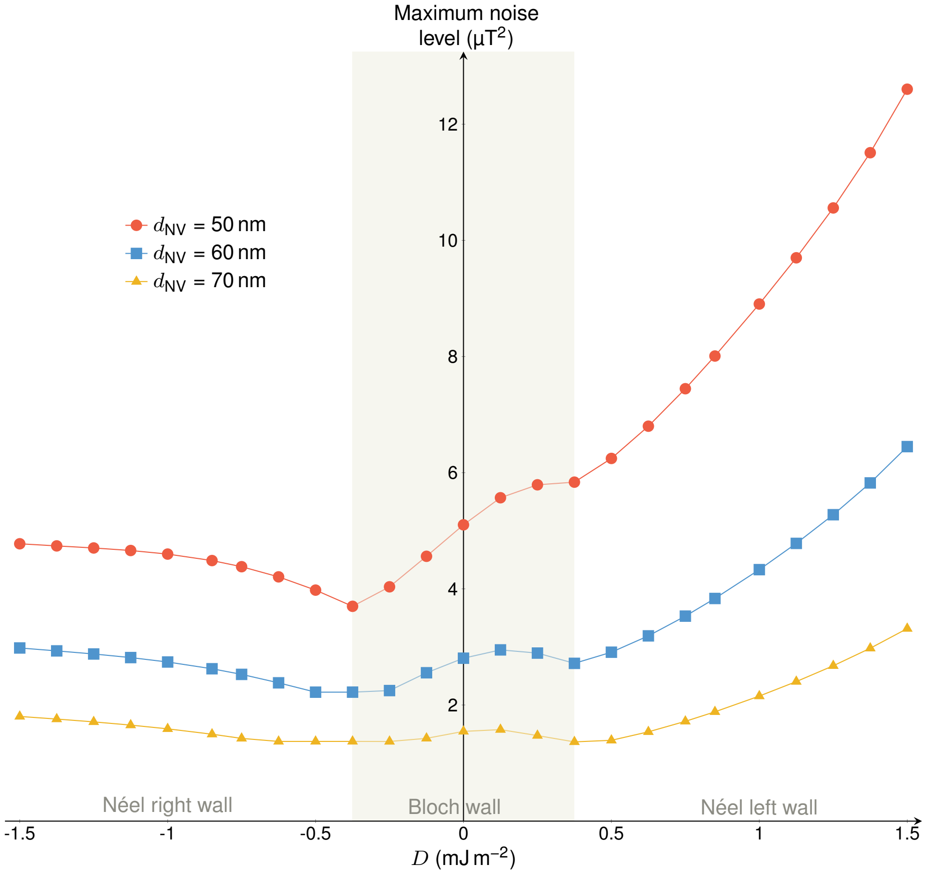


FIG. S3. Calculated maximal noise level at 2.87 GHz and at various values of $d_{NV}$ expected above the surface of the film hosting a domain wall, when varying the DMI constant $D$. Note that high values of $|D|$ are unphysical, as the domain wall becomes unstable.

## IV. SAMPLE PREPARATION

In this section we describe the sample preparation of the synthetic antiferromagnetic (SAF) and the single ferromagnetic layer stacks grown on membranes used along this work. Details about the other SAF sample (Figs 2 and 4 of the main text) are provided in ref. [3].

The samples were deposited by sputtering deposition on 20 to 30 nm thick SiN membranes with the following composition Ta(3)/Pt(3)/Co($t$)/Ru(0.85)/Pt(0.45)/Co($t$)/Ru(0.6)/Ta(1.5) and Ta(3)/Pt(3)/Co(1.35)/Ru(0.85)/Ta(2) respectively (where numbers in parenthesis are the nominal thicknesses in nanometers). The SAF structure is grown on a 100 mm wafer using off-axis deposition, such that the Co thickness varies from 1.4 to 1.9 nm. The Ru spacer thickness is choosen to be 0.85 nm in order to tune the RKKY interaction to be the maximally antiferromagnetic. Moreover, the interlayer Pt thickness is choosen to be 0.45 nm to achieve a large RKKY coupling and obtain a similar anisotropy in both ferromagnetic layers. The single ferromagnetic stack has been deposited using on-axis technique where the Co thickness is optimized to exhibit worm-like domains of few microns. A MOKE image of this sample is shown in Fig. S4. Note also that all stacks are capped with a Ta thin layer to protect them from oxidation.

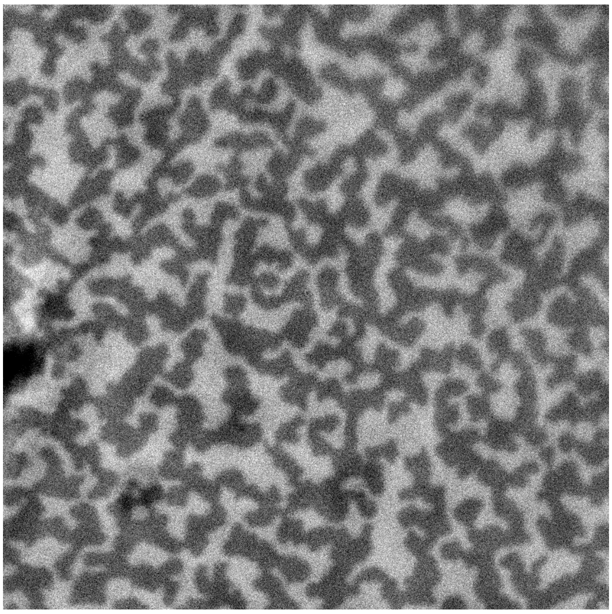

FIG. S4. MOKE image ($50 \times 50\,\mu m^2$) of the single ferromagnetic layer grown on a membrane, measured in the absence of applied magnetic field. Worm-like domains of a few microns are present.

## V. CALIBRATION OF THE DIAMOND PROBES

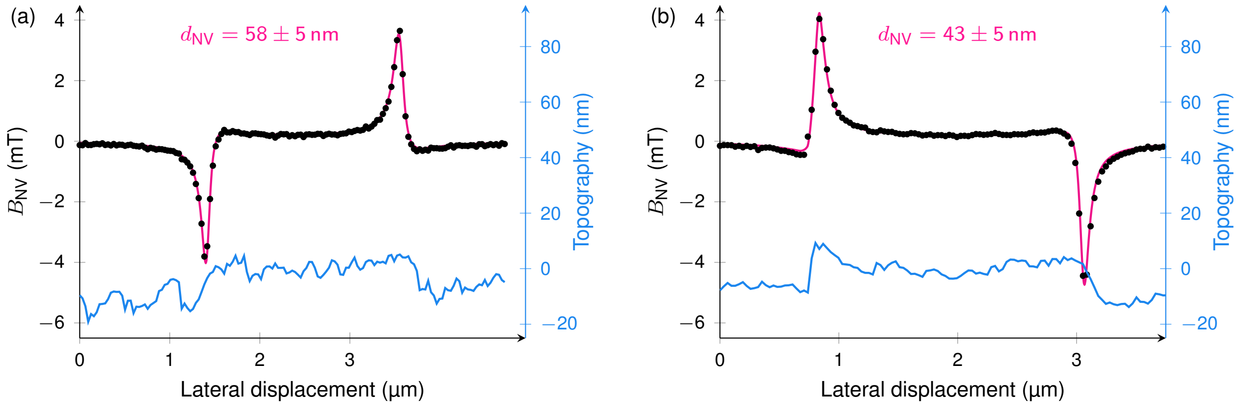


FIG. S5. Calibration experiments for the two probes used in Fig. 2 of the main text. The probe (a) was used to investigate the Néel left stack, while the probe (b) was used to probe the Néel right textures through the membrane. These measurements are performed on a 2 µm-wide ferromagnetic stripe, with the following composition: $TaN_{0.7\%}$(1 nm)|$Co_{20}Fe_{60}B_{20}$(1 nm)|MgO(2 nm) and analyzed following the method detailed in ref. [4]. The indicated values of $d_{\rm NV}$ take into account the 2 nm-thick MgO capping layer.

## VI. MICROMAGNETICS SIMULATIONS

### A. Geometry and parameters

The magnetic noise spectrum was investigated numerically using the micromagnetics code `MuMax3` [5, 6]. The code performs a numerical time integration using the finite difference method of the Landau-Lifshitz equation with Gilbert damping,

$$\frac{d\mathbf{m}}{dt} = -|\gamma_0|\mathbf{m} \times \mathbf{H}_{\text{eff}} + \alpha \mathbf{m} \times \frac{d\mathbf{m}}{dt}, \tag{1}$$

where $\|\mathbf{m}(\mathbf{r}, t)\| = 1$ is a unit vector representing the orientation of the magnetization field, $\gamma_0 = \mu_0 g \mu_B/\hbar$ is the gyromagnetic constant, and $\alpha$ is the Gilbert damping constant. With $M_s$ denoting the saturation magnetization, the effective field, $\mathbf{H}_{\text{eff}} = -(1/\mu_0 M_s)\delta U/\delta \mathbf{m}$, represents a variational derivative of the total magnetic energy $U$ with respect to the magnetization, with $U$ containing contributions from the Zeeman, nearest-neighbor Heisenberg exchange, Dzyaloshinskii-Moriya, and dipole-dipole interactions along with a uniaxial anisotropy with an easy axis along $\hat{\mathbf{z}}$, perpendicular to the film plane. We account for finite temperatures by adding a random thermal field, $\mathbf{h}_{\text{th}}$, to the effective field, $\mathbf{H}_{\text{eff}} \to \mathbf{H}_{\text{eff}} + \mathbf{h}_{\text{th}}$. This random field represents a Gaussian white noise with the spectral properties

$$\langle h_{\text{th},i}(\mathbf{r}, t)\rangle = 0, \ \langle h_{\text{th},i}(\mathbf{r}, t) h_{\text{th},j}(\mathbf{r}', t')\rangle = \frac{2\alpha k_B T}{\mu_0 \gamma_0 M_s}\delta_{ij}\delta(\mathbf{r} - \mathbf{r}')\delta(t - t'), \tag{2}$$

where $i, j = x, y, z$ represent the different Cartesian components of the field.

For the ferromagnetic film shown in Figure 1 of the main text, we used a saturation magnetization of $M_s = 1.2$ MA/m, an exchange constant of $A = 20$ pJ/m, a uniaxial anisotropy constant of $K_u = 0.935$ MJ/m$^3$, and a variable interfacial Dzyaloshinskii-Moriya interaction constant $D$. The simulated film is represented by a rectangular box with dimensions of $2000 \times 2000 \times 1.5$ nm$^3$, which is discretized using $512 \times 512 \times 1$ finite difference cells.

For the synthetic antiferromagnet considered in Figure 4, we used the same values for $M_s$ and $A$. For the top ferromagnetic layer, we used a base value of $K_{u,\text{top}} = 0.921$ MJ/m$^3$, while for the bottom ferromagnetic layer, we used a base value of $K_{u,\text{bot}} = 0.935$ MJ/m$^3$ and . To model disorder, we used Voronoi tessellation with cells of an average size of 20 nm to represent grains. For each grain $n$, $K_{u,n}$ is assigned a random value drawn from a normal distribution centered on the base anisotropy with a width representing a 1% fluctuation. An antiferomagnetic exchange interaction (RKKY) between the two layers of $-0.22$ mJ/m$^2$ was used.

In order to compare Néel and Bloch skyrmions with similar sizes, we employed the following approach. For the Néel type skyrmions, we used $D_{\text{top}} = \pm 0.425$ mJ/m$^2$ and $D_{\text{bot}} = \pm 0.850$ mJ/m$^2$ for the *interfacial* Dzyaloshinskii-Moriya constant for the top and bottom layer, respectively, with positive values resulting in left-handed textures. For the Bloch type skyrmions, lower values of $D_{\text{top}} = \pm 0.334$ mJ/m$^2$ and $D_{\text{bot}} = \pm 0.667$ mJ/m$^2$ for the *bulk* Dzyaloshinskii-Moriya constant were used in order to compensate for the dipolar interaction, which favors Bloch-type textures.

The synthetic antiferromagnet comprises a trilayer structure with dimensions of $1000 \times 1000 \times 4.5$ nm$^3$ and discretized with $512 \times 512 \times 3$ finite difference cells. The spacer layer is taken to be nonmagnetic and represented by empty cells in the simulation.

### B. Spin wave dispersion relations

The spin wave dispersion relations in Figs. 1(b), 1(c), and S2 were calculated for a domain wall running along the $x$ direction, while translational invariance was assumed along the $y$ direction by applying periodic boundary conditions. The dispersion relations were constructed from the transient response to a time-dependent magnetic field of the form $\mathbf{b}_{\rm rf}(y,t) = b_0(t)\,[\cos(k_n y)\hat{\mathbf{u}}(x) + \sin(k_n y)\hat{\mathbf{v}}(x)]$, where $\hat{\mathbf{u}}, \hat{\mathbf{v}}$ represent the transverse directions to the static magnetization. $b_0(t) = \sin(\pi\nu t)/\pi\nu t$ is a sinc function with $\nu = 150$ GHz and amplitude of 1 mT, while $k_n = 2\pi n/N_y$ is a quantized wave vector along the propagation direction, $y$. For each value of the wave vector $k_n$, $b_{\rm rf}(t)$ was applied to the system starting from the initial relaxed magnetic configuration and the damped magnetic response was simulated over 100 ns. The power spectrum was then computed from the Fourier transform of this magnetic response, taken at positions $x_d$ and $x_w$ to obtain the dispersion within the domain and at the wall center, respectively, as shown in Fig. 1(a).

### C. Simulated magnetic noise spectra

To estimate the relevant magnetic noise spectrum for the relaxometry measurements, we simulated the magnetic response to thermal fluctuations by computing the dynamics subject to a random spatial field with a harmonic time dependence at a frequency of 2.87 GHz. The idea is to estimate the power spectrum of magnetic fluctuations at 2.87 GHz by computing the magnetic susceptibility at this frequency. This random field varies between each finite difference cell, where its orientation is drawn from a uniform distribution over the unit sphere (i.e., the $z$ component is taken to be a random value between $[1,-1]$ and the azimuthal angle is drawn randomly from the interval $[0,2\pi)$), while its magnitude is drawn from a Gaussian distribution centred at zero with a variance of 1 mT$^2$. The random field is applied to a relaxed magnetic state.

The noise map is computed as follows. For a given realisation $i$ of the random magnetic field, the ensuing dynamics is calculated over one period of the 2.87 GHz excitation and the micromagnetic state is recorded. We then compute the deviation in the stray magnetic field with respect to the relaxed state $\mathbf{m}_0$, $\delta\mathbf{B}_i = \mathbf{B}_i - \mathbf{B}_0$, at different distances from the single or multilayer, which models the field seen by the NV center at different probe heights. The square of the magnitude of the projection of this field along the direction perpendicular to the NV axis, $\|\delta\mathbf{B}_{\perp,i}\|^2$, is then recorded at each position of the simulation grid. The quantities in Figs. 1(d), 1(f), 1(g), 4(c)-4(f), and S3 represent an average of $\|\delta\mathbf{B}_{\perp,i}\|^2$ over 500 different realisations of the random driving field.

---


[1] J.-P. Tetienne, L. Rondin, P. Spinicelli, M. Chipaux, T. Debuisschert, J.-F. Roch, and V. Jacques, Magnetic-field-dependent photodynamics of single NV defects in diamond: An application to qualitative all-optical magnetic imaging, New Journal of Physics **14**, 103033 (2012).

[2] F. Garcia-Sanchez, P. Borys, R. Soucaille, J.-P. Adam, R. L. Stamps, and J.-V. Kim, Narrow Magnonic Waveguides Based on Domain Walls, Physical Review Letters **114**, 247206 (2015).

[3] V. T. Pham, N. Sisodia, I. Di Manici, J. Urrestarazu-Larrañaga, K. Bairagi, J. Pelloux-Prayer,

R. Guedas, L. D. Buda-Prejbeanu, S. Auffret, A. Locatelli, T. O. Menteş, S. Pizzini, P. Kumar, A. Finco, V. Jacques, G. Gaudin, and O. Boulle, Fast current-induced skyrmion motion in synthetic antiferromagnets, Science **384**, 307 (2024).

[4] T. Hingant, J.-P. Tetienne, L. J. Martínez, K. Garcia, D. Ravelosona, J.-F. Roch, and V. Jacques, Measuring the Magnetic Moment Density in Patterned Ultrathin Ferromagnets with Submicrometer Resolution, Physical Review Applied **4**, 014003 (2015).

[5] A. Vansteenkiste, J. Leliaert, M. Dvornik, M. Helsen, F. García-Sánchez, and B. V. Waeyenberge, The design and verification of MuMax3, AIP Advances **4**, 107133 (2014).

[6] J. Leliaert, J. Mulkers, J. D. Clercq, A. Coene, M. Dvornik, and B. V. Waeyenberge, Adaptively time stepping the stochastic Landau-Lifshitz-Gilbert equation at nonzero temperature: Implementation and validation in MuMax 3, AIP Advances **7**, 125010 (2017).
